# Supplementary material for: Towards High-fidelity Head Blending with Chroma Keying for Industrial Applications
Source: arXiv:2411.00652 source file (2024-11-01)
Supplement: Supplementary file 1 [file fig_supp_qualitative.tex]

\begin{figure*}[t]
\begin{center}
\includegraphics[width=2.1\columnwidth]{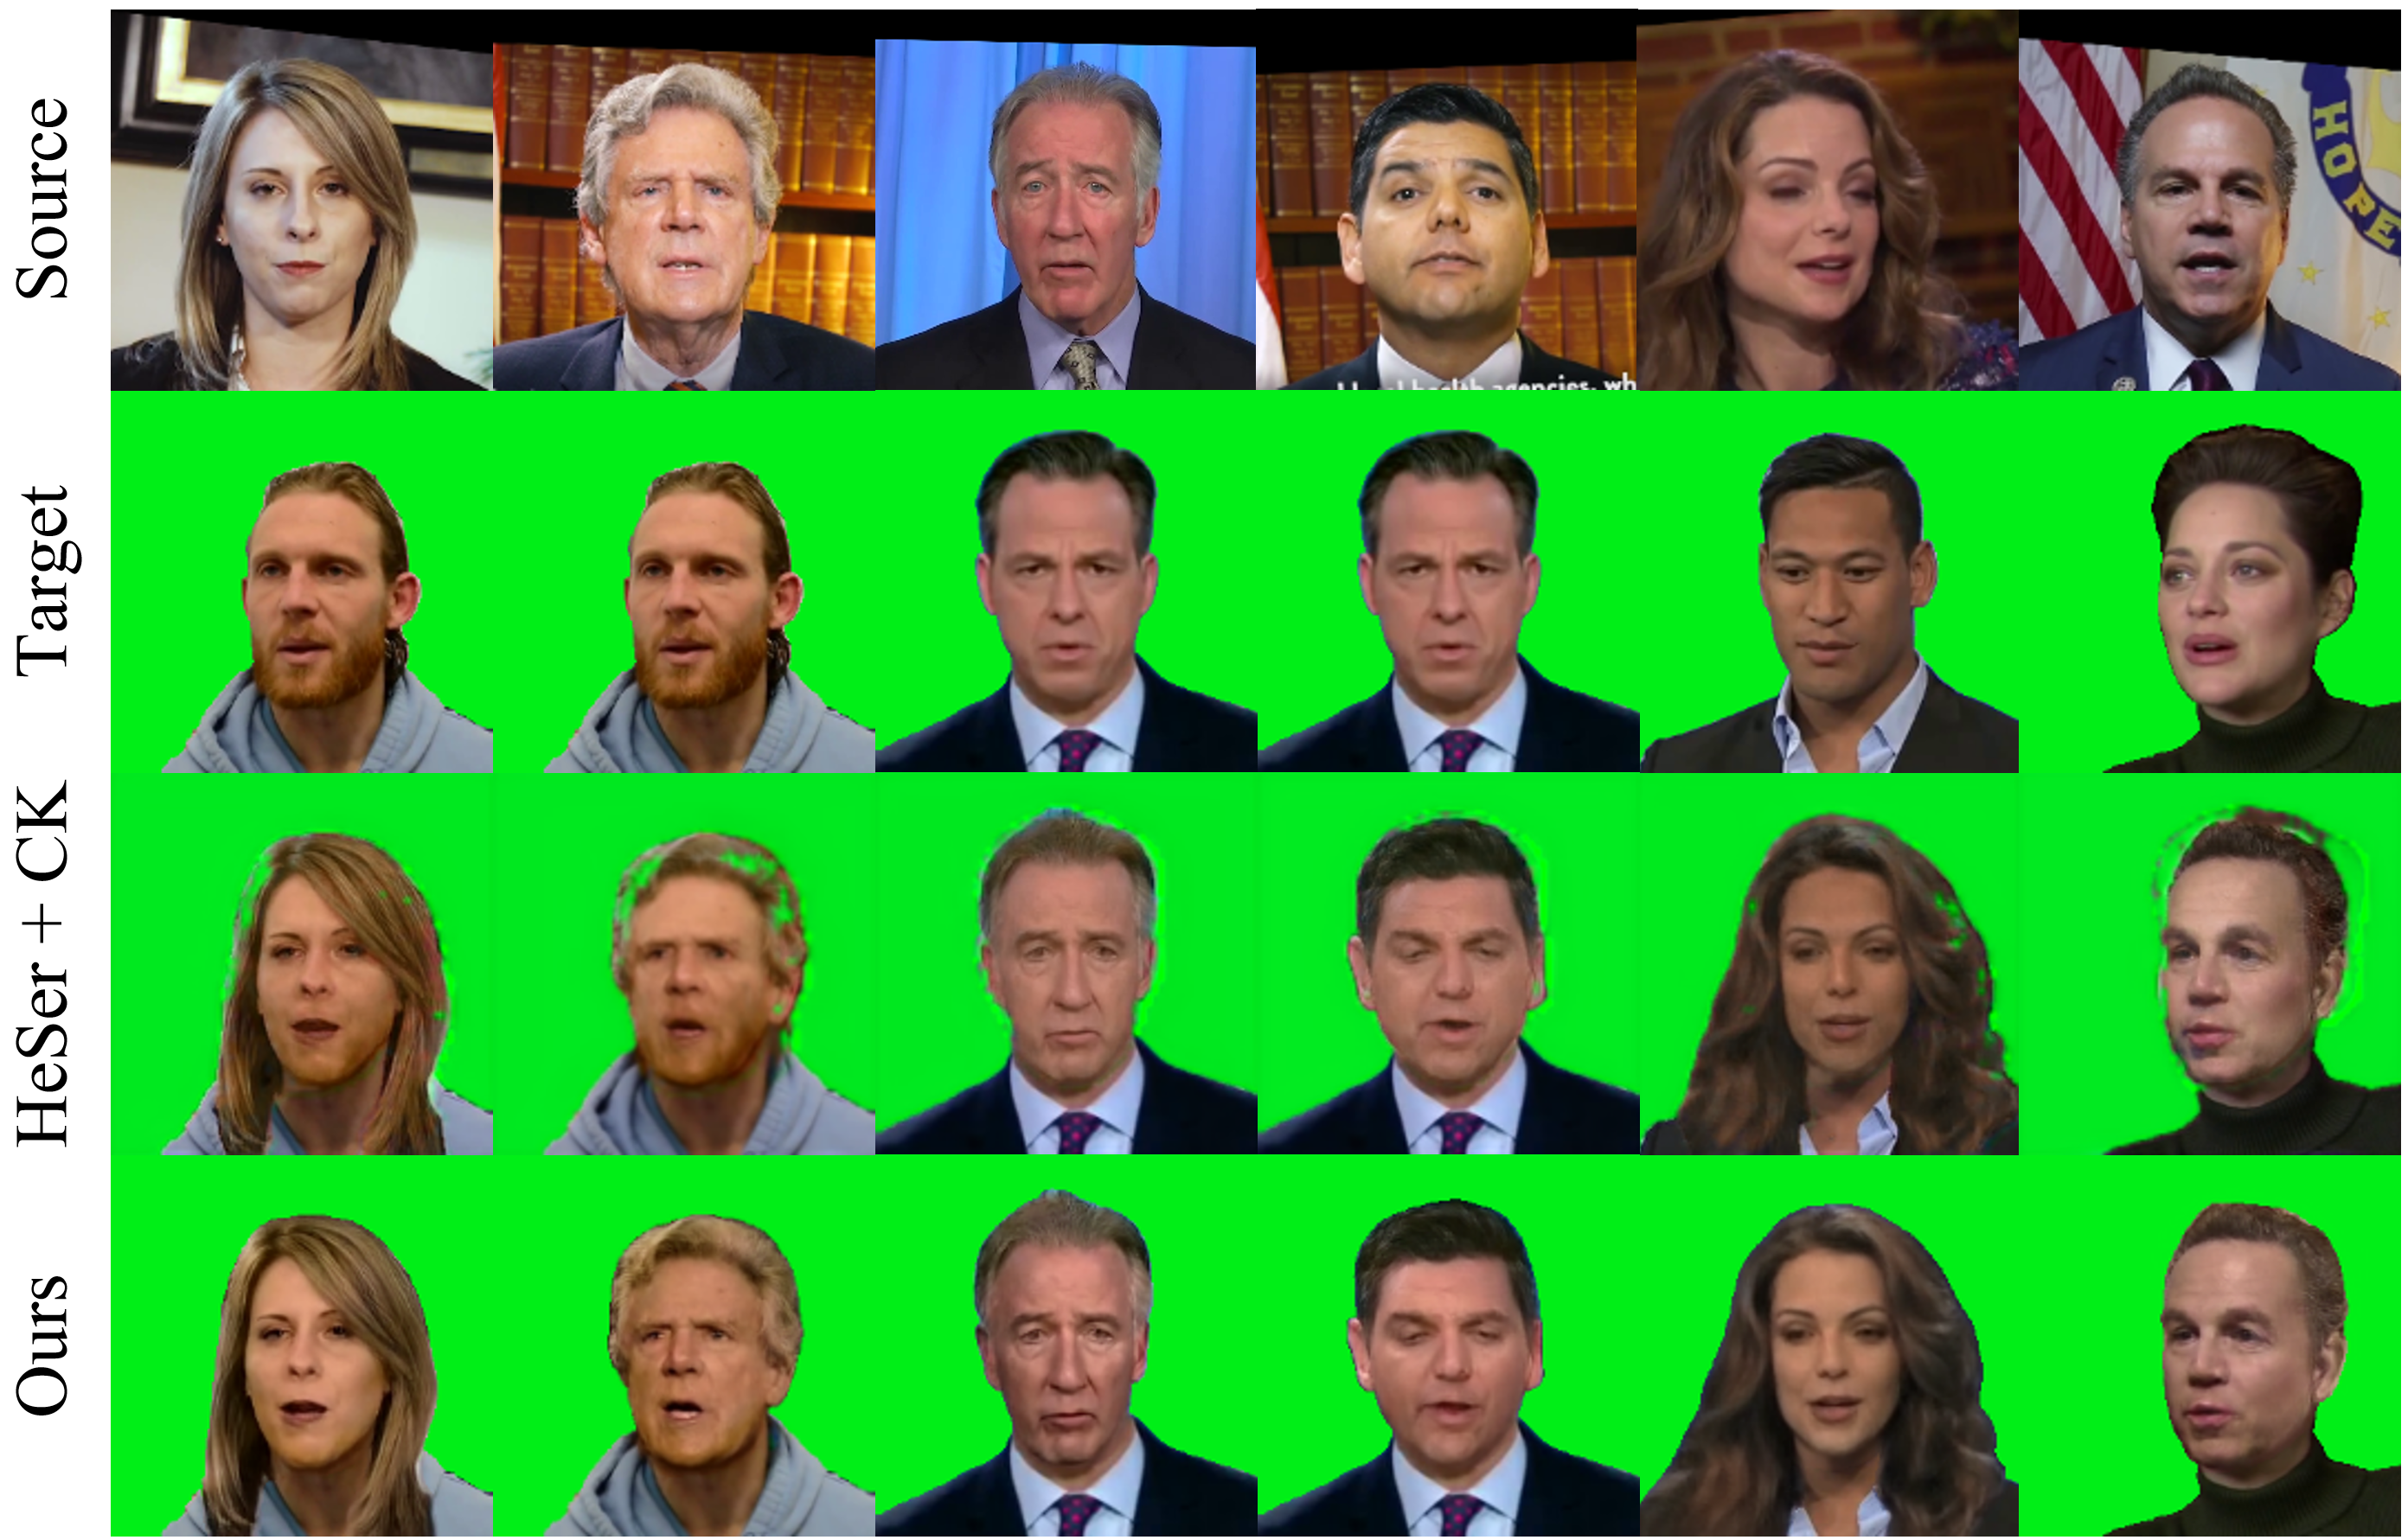}
\end{center}
\caption{
Qualitative head swapping results in green screen scenario. Chroma-HS (Ours) shows high-fidelity head-swapped images compared to the HeSer~\cite{shu2022few} with our chroma keying.
}
\label{fig:suppqualitative}
\end{figure*}
